# Supplementary material for: Scalable Reinforcement-Learning-Based Neural Architecture Search for Cancer Deep Learning Research
Source: arXiv:1909.00311 source file (2019-09-01)
Supplement: Supplementary file 1 [file appendix.tex]

Figures \ref{fig:combo_baseline}, \ref{fig:uno_baseline},  \ref{fig:nt3_baseline} show respectively the manually designed neural network for 
\combo, \uno, and \ntthree benchmarks.

\begin{figure}
    \centering
    \includegraphics[width=0.45\textwidth]{img/combo_default.pdf}
    \caption{Baseline neural network for \combo}
    \label{fig:combo_baseline}
\end{figure}

\begin{figure}
    \centering
    \includegraphics[width=0.45\textwidth]{img/uno_default.pdf}
    \caption{Baseline neural network for \uno}
    \label{fig:uno_baseline}
\end{figure}

\begin{figure}
    \centering
    \includegraphics[width=0.35\textwidth]{img/nt3_default.pdf}
    \caption{Baseline neural network for \ntthree}
    \label{fig:nt3_baseline}
\end{figure}
